# Supplementary material for: Solving Robust Markov Decision Processes: Generic, Reliable, Efficient
Source: arXiv:2412.10185 source file (2024-12-13)
Supplement: Supplementary file 1 [file 15_appendix_poly_lra_pseudocode.tex]

\begin{algorithm}[tb]
	\caption{Bounded value iteration for RMDP}
	\label{alg:3-app-LRA}
	\textbf{Input}: RMDP $\RMDP=(\States,\Actions,\rmdptransitions,\rew)$, initial state $s_0$ and desired precision $\varepsilon>0$\\
	\textbf{Output}: lower and upper bounds $\lb$ and $\ub$ on the long-run average reward $\val_{\RMDP}^\opt$
	\begin{algorithmic}[1] 
		
		\FORALL{$s\in S$} 
		\STATE $\lb_0(s)\gets 0$, $x_0(s) \gets 0$, $\ub_0(s) \gets \max_{s\in\States}\rew(s)$
		\ENDFOR
		\STATE $i \gets 0$
		
		\WHILE{$\ub(s_i)-\lb(s_i) > \varepsilon$} 
		\FORALL{$s\in S$} 
		\STATE 	$x_{i+1}(s) \gets \opt_{a\in\Actions(s)} \rew(s,a)~+$
		
		$\quad\quad\quad\overline{\opt}_{\mdptransitions(s,a)\in\rmdptransitions(s,a)} \sum_{s' \in \States} \mdptransitions(s,a)(s') x_i(s')$
		\STATE 	$\lb_{i+1}(s) \gets \opt_{a\in\Actions(s)}$
		
		$\quad\quad\quad\overline{\opt}_{\mdptransitions(s,a)\in\rmdptransitions(s,a)} \sum_{s' \in \States} \mdptransitions(s,a)(s') \lb_i(s')$
		\STATE 	$\ub_{i+1}(s) \gets \opt_{a\in\Actions(s)}$
		
		$\quad\quad\quad\overline{\opt}_{\mdptransitions(s,a)\in\rmdptransitions(s,a)} \sum_{s' \in \States} \mdptransitions(s,a)(s') \ub_i(s')$
		\ENDFOR
		\STATE $\FINDANDDEFLATE$
		\STATE $i \gets i+1$
		\ENDWHILE
		\STATE \textbf{return} $(\lb_i,\ub_i)$
	\end{algorithmic}
\end{algorithm}
